# Supplementary material for: Deep Reinforcement Learning for Safe Landing Site Selection with Concurrent Consideration of Divert Maneuvers
Source: arXiv:2102.12432 source file (2021-02-24)
Supplement: Supplementary file 1 [file Appendix.tex]

\appendix
\section*{Appendix: Title here}
Each appendix is its own section with its own section heading. The title of each appendix section is preceded by ``APPENDIX: '' as illustrated above, or ``APPENDIX A: '', ``APPENDIX B: '', \emph{etc}., when multiple appendixes are necessary. Appendices are optional and normally go after references; however, appendices may go ahead of the references section whenever the word processor forces superscripted endnotes to the very end of the document. The contents of each appendix must be called out at least once in the body of the manuscript.

\subsection*{Miscellaneous Physical Dimensions}
The page size shall be the American standard of 8.5 inches by 11 inches (216 mm x 279 mm). Margins are as follows: Top -- 0.75 inch (19 mm); Bottom -- 1.5 inches (38 mm); Left -- 1.25 inches (32 mm); Right -- 1.25 inch (32 mm). The title of the manuscript starts one inch (25.4 mm) below the top margin. Column width is 6 inches (152.5 mm) and column length is 8.75 inches (222.5 mm). The abstract is 4.5 inches (114 mm) in width, centered, justified, 10 point normal (serif) font.
